# Supplementary material for: IRFL: Image Recognition of Figurative Language
Source: arXiv:2303.15445 source file (2023-11-25)
Supplement: Supplementary file 1 [file 100B_dataset_supplementary_materials.tex]

\begin{enumerate}
  \item After the review process is complete, dataset documentation, metadata, and download instructions will be released.
  \item Intended uses: We hope researchers will use our benchmarks to evaluate Vision and Language models. We also hope that our pipeline and dataset will inspire future work on creating extensive multimodal datasets of other figures of speech.
  \item Author statement: We bear all responsibility in case of violation of rights in using our benchmark. 
  \item Licenses: Dataset is licensed under CC-BY 4.0 license \url{https://creativecommons.org/licenses/by/4.0/legalcode}.
\end{enumerate}
